# Supplementary material for: Adapting Knowledge Prompt Tuning for Enhanced Automated Program Repair
Source: arXiv:2504.01523 source file (2025-04-02)
Supplement: Supplementary file 1 [file appendix.tex]

% \begin{table*}[h!]
%   \centering
%   \small
%   \caption{Results of various advanced prompts on CodeT5+ 220m }
%   \label{tab:result}
%   \renewcommand{\arraystretch}{1}
%   \begin{tabular}{ccc|cc|cc|cc} 
%     \toprule 
%     &  \multicolumn{2}{c|}{\textbf{Hard advanced prompt}}  & \multicolumn{2}{c|}{\textbf{hard token-infused soft prompts}} &  \multicolumn{2}{c|}{\textbf{knowledge-infused soft prompts }} & \multicolumn{2}{c}{\textbf{pure soft prompts}}  \\
%         \midrule 
%     &  CodeBLEU & CP  &  CodeBLEU & CP &  CodeBLEU & CP &  CodeBLEU & CP  \\
%         \midrule 
%     & \multicolumn{8}{c}{\textbf{Defects4j}}   \\

%     \midrule 
% 1  &  68.27	& 2/19	& 69.25&1/19&69.15&1/19& 69.02&1/19\\
% 2 & 70.38 &	1/19	&70.06 &1/19&68.2&1/19&	69.16&1/19\\
% 3 & 69.49 &	1/19	&66.56 &1/19&68.47&1/19&	69.16&1/19\\
% 4 & 71.64 & 1/19	& 69.21&1/19&67.28&1/19&69.24&1/19\\

%     \midrule 
% & \multicolumn{8}{c}{\textbf{Quixbugs-Python}}   \\
%     \midrule 
% 1  & 84.17 & 0/4 &83.79&0/4&83.79&0/4&83.79&0/4\\
% 2  & 82.31 &0/4 &80.24&0/4&81.24&0/4&83.23&0/4\\
% 3  & 70.56 & 0/4&83.23&0/4&84.17&0/4&79.98&0/4\\
%     \midrule 
% & \multicolumn{8}{c}{\textbf{Quixbugs-Java}}   \\
%     \midrule 
% 1  & 92.94 & 0/4&92.32&0/4&92.94&0/4&86.68& 0/4\\
% 2  & 86.68 & 0/4&92.94&0/4&86.68&0/4&86.68& 0/4\\
% 3  & 92.94 & 0/4&92.94&0/4&92.94&0/4&86.68&0/4\\
%     \midrule 
%     & \multicolumn{8}{c}{\textbf{ManyBugs}}   \\
%     \midrule 
% 1  & 70.36 & 0/14 &60.82&0/14&61.46&0/14&60.79&0/14\\
%     \midrule 
%     & \multicolumn{8}{c}{\textbf{ManySStuBs4J}}   \\
%     \midrule 
% 1  & 95.23 & 33/43 &97.55& 35/43&97.4& 33/43&97.32& 33/43\\
% 2  &  96.37& 33/43 &98.9& 41/43&97.89& 38/43&97.14& 32/43\\
% 3  & 98.12 & 39/43 &98.18& 39/43&98.9& 41/43&97.32& 33/43\\
% \bottomrule
%   \end{tabular}
% \end{table*}
